# Supplementary material for: Narrow inhomogeneous distribution of spin-active emitters in silicon carbide
Source: arXiv:2103.06101 ancillary file (2021-03-12)
Supplement: Supplementary file 1 [file Supplementary_Material.pdf]

# Supplementary Material for:
# Narrow inhomogeneous distribution of spin-active emitters in silicon carbide

Roland Nagy[1,2], Durga Bhaktavatsala Rao Dasari[2], Charles Babin[2], Di Liu[2], Vadim Vorobyov[2], Matthias Niethammer[2], Matthias Widmann[2], Tobias Linkewitz[2], Izel Gediz[2], Rainer Stöhr[2], Heiko B. Weber[3], Takeshi Ohshima[4], Misagh Ghezellou[5], Nguyen Tien Son[5], Jawad Ul-Hassan[5], Florian Kaiser[2,*] and Jörg Wrachtrup[2]

[1] *Department Elektrotechnik-Elektronik-Informationstechnik (EEI), Friedrich-Alexander-Universität Erlangen-Nürnberg (FAU), 91058 Erlangen (Germany)*
[2] *3rd Institute of Physics, IQST, and Research Center SCoPE, University of Stuttgart, 70569 Stuttgart (Germany)*
[3] *Department of Physics, Friedrich-Alexander-Universität Erlangen-Nürnberg (FAU), 91058 Erlangen (Germany)*
[4] *National Institutes for Quantum and Radiological Science and Technology, Takasaki, Gunma 370- 1292 (Japan)*
[5] *Department of Physics, Chemistry and Biology, Linköping University, SE-58183 Linköping (Sweden)*

## REQUIRED NUMBER OF DEFECTS UNTIL FINDING OVERLAPPING LINES

The theoretical fit in Fig. 2(d) is obtained in analogy to the popular birthday paradox [1]. Consider that two randomly chosen emitters have a spectral overlap probability $p$ within a given frequency separation. Then, the probability that $n$ emitters do not show any spectral overlap is $\bar{P} = n!\binom{p^{-1}}{n}/\left(\frac{1}{p}\right)^n$. In general, $p^{-1}$ is not an integer number, thus requiring to extend all appearing factorials with the gamma function, i.e. $x! = \Gamma(x+1)$. The number $n$ of defects to be investigated until at least one pair of overlapping lines is found with a probability exceeding 50% is then obtained by solving:

$$0.5 \leq 1 - \bar{P}. \tag{S1}$$

To plot the red line in Fig. 2(d), we re-scale the x-axis by the relationship between overlap probability and line separation (red line linear fit in Fig. 2(c)). Experimentally, we found that the overlap probability increases with a slope of 1.12(3)% per line separation of 29 MHz. The blue dots in Fig. 2(d) are obtained by solving equation (S1) for the measured overlap probabilities in Fig. 2(c).

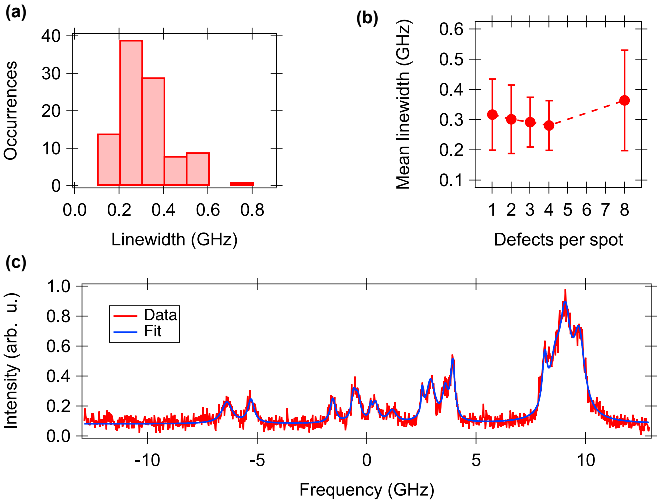


FIG. S1. Optical linewidth analysis. (a) Distribution of the observed absorption linewidths (full width at half maximum) for 50 defects. (b) Average observed linewidths as a function of the local defect density. Error bars represent one standard deviation. (c) Exemplary data set for a spot containing eight defects. The fit is based on a multi-Lorentzian function with 16 peaks.

## DISTRIBUTION OF OPTICAL LINEWIDTHS

A histogram of all observed optical linewidths in shown in FIG. S1(a). The average full width at half maximum is found to be 316 MHz with a standard deviation of 122 MHz. The distributions for the $A_1$ and $A_2$ lines are very similar and thus not shown separately. FIG. S1(b) shows the average linewidth as a function of the number of defects within a diffraction-limited spot. In our study, we found 21 spots with a single defect, 7 spots with two defects, 1 spot with three defects, 1 spot with four defects, and 1 spot with eight defects. The data shows that there is no significant increase in the optical linewidth as a function of the local defect density. We conclude therefore that the minimum achievable linewidth is mainly limited by global 4H-SiC crystal parameters, such as a slightly elevated Fermi level due to an increased nitrogen concentration in the $5 \cdot 10^{13}\,\mathrm{cm}^{-3}$ range. FIG. S1(c) shows an exemplary set of absorption line measurement data and the associated fit, here for the spot that contains eight h-$V_{Si}$ centres.

## SPATIAL DISTRIBUTION OF THE OPTICAL ABSORPTION LINES

To evaluate whether there is a spatial distribution in the optical absorption lines, we split the data sets into four sections. The sections are chosen according to the y-axis coordinate in Fig. 1(a) in the main text. Quartile 1 comprises defects with a y-coordinate $0\,\mu\mathrm{m} \leq \mathrm{y} <$

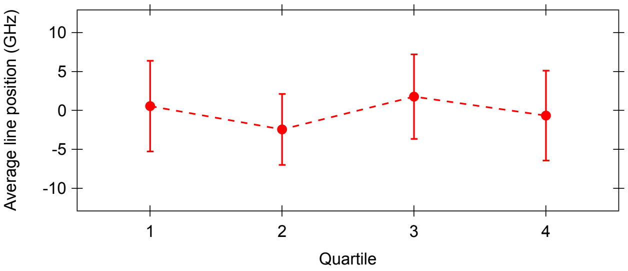


FIG. S2. Spatial distribution of absorption line positions for multiple defects in four different quartiles. Erorr bars denote one standard deviation. The dashed line is a guide to the eye.

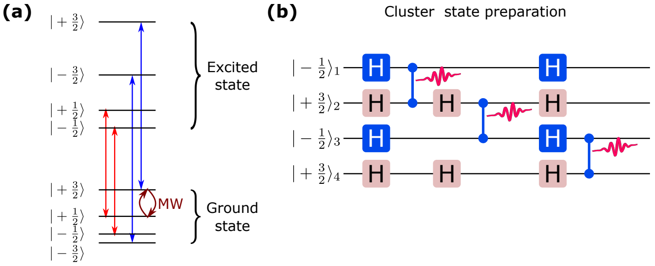


FIG. S3. (a) Energy level scheme of h-$V_{Si}$ centres in order to generate cluster states. Application of an external magnetic field lifts the ground and excited state degeneracy. MW drive is used for deterministic spin initialisation. (b) Protocol for the generation of spin cluster states. The blue (pink) colored Hadamard gates (H) perform rotations in the independent subspace $\{|-\frac{3}{2}\rangle;|-\frac{1}{2}\rangle\}$ ($\{|+\frac{3}{2}\rangle;|+\frac{1}{2}\rangle\}$). In each step along the circuit diagram, gates of identical color are applied simultaneously.

$3\,\mu$m. Quartile 2 comprises defects with a y-coordinate $3\,\mu\mathrm{m} \leq \mathrm{y} < 6\,\mu$m. Quartile 3 comprises defects with a y-coordinate $6\,\mu\mathrm{m} \leq \mathrm{y} < 9\,\mu$m. And quartile 4 comprises defects with a y-coordinate $9\,\mu\mathrm{m} \leq \mathrm{y} < 12\,\mu$m. Each quartile's average optical absorption line position is shown in FIG. S2. The data reveals no significant drift, such that we conclude that the absorption line distribution is similar across the entire sample.

## GENERATION OF MULTI-SPIN CLUSTER STATES

To detail the generation of spin cluster states, we consider the same four defect array as shown in FIG. 4(a) in the main text. In addition, we take advantage of the full potential of the four-level ground state. To this end, we consider an external magnetic field that lifts the ground (and excited) state degeneracy (see FIG. S3(a)). We use the same pairwise spin initialisation procedure as described in the main text for the GHZ states, however, we apply an additional common MW drive in the ground state to continuously mix the spin sublevels $|+\frac{1}{2}\rangle$ and $|+\frac{3}{2}\rangle$. As demonstrated in Ref. [2], this eventually leads to high-fidelity spin initialisation: $|\psi_{0,\mathrm{c}}\rangle = |-\frac{1}{2}\rangle_1|-\frac{3}{2}\rangle_2|-\frac{1}{2}\rangle_3|-\frac{3}{2}\rangle_4$. Subsequently applying a MW $\pi$-pulse on the spin transition $|+\frac{1}{2}\rangle \leftrightarrow |-\frac{1}{2}\rangle$ results in $|\psi_{1,\mathrm{c}}\rangle = |+\frac{1}{2}\rangle_1|-\frac{3}{2}\rangle_2|+\frac{1}{2}\rangle_3|-\frac{3}{2}\rangle_4$. This state is particularly interesting as it allows to independently manipulate all even-numbered defects in the spin subspace $\{|+\frac{1}{2}\rangle;|+\frac{3}{2}\rangle\}$ and all odd-numbered defects in $\{|-\frac{3}{2}\rangle;|-\frac{1}{2}\rangle\}$. By applying the circuit shown in FIG. S3(b), we project the initial four-spin state to the entangled state:

$$|\psi_{\mathrm{C}}\rangle = \frac{1}{2}\Big(|\uparrow\rangle_1|+\rangle_2|\uparrow\rangle_3|\uparrow\rangle_4 + |\uparrow\rangle_1|+\rangle_2|\downarrow\rangle_3|\downarrow\rangle_4 + |\downarrow\rangle_1|-\rangle_2|\uparrow\rangle_3|\uparrow\rangle_4 - |\downarrow\rangle_1|-\rangle_2|\downarrow\rangle_3|\downarrow\rangle_4\Big). \quad \text{(S2)}$$

Up to a local unitary, this is the well-known four-qubit cluster state [3]. In equation S2, we have used the following identities: $|\pm\frac{1}{2}\rangle_i \equiv |\uparrow\rangle_i$, $|\pm\frac{3}{2}\rangle_i \equiv |\downarrow\rangle_i$, and $|\pm\rangle_i = (|\uparrow\rangle_i \pm |\downarrow\rangle_i)/\sqrt{2}$ with $i = 1, 2, 3, 4$.

## PROBABILISTIC ENTANGLEMENT GENERATION

As described in the main text, the GHZ/cluster state generation is probabilistic in nature as it is conditioned on single photon detection events. Considering a finite detection efficiency $\eta$ for a single photon, the probability for detecting the correct single-photon event in both one and two-photon cases is given by $P = P_{1,1}/(P_{1,1}+P_{1,2})$, where $P_{1,k}$ is the probability of detecting a single photon in a $k-$photon emission event. Substituting for $P_{1,1} = \eta$, $P_{1,2} = 2\eta(1-\eta)$, one immediately finds that the fidelity of generated spin-pair after single-photon detection is $F^{(2)}_{\mathrm{GHZ}} = 1/(3-2\eta)$. Extending this for the case of $n$-emitter case this fidelity simplifies to $F^{(n)}_{\mathrm{GHZ}} = 1/[2(n-1)(1-\eta)+1]$, which is shown in FIG. S4(a).

In direct analogy, we repeat the analysis for the cluster state generation protocol. For a direct generation of a four-qubit cluster state, the fidelity is found to be $F^{(4)}_{\mathrm{C}} = \frac{1}{(3-2\eta)(4-4\eta)(5-4\eta)}$. From the multi-emitter states, we also extract the purity, $\mathcal{P} = \mathrm{Tr}(\rho^2)$ of the heralded final states as a function of the detection efficiency $\eta$. The fidelity and purity for the four-qubit cluster generation protocol are shown FIG. S4(b).

## SPIN ASSISTED MULTI-PHOTON ENTANGLEMENT

As described earlier, a tunable interaction of the excitation laser with a target emitter allows for the generation of $N$-spin GHZ or cluster states. Here, we show that one can also take advantage of the spin control to

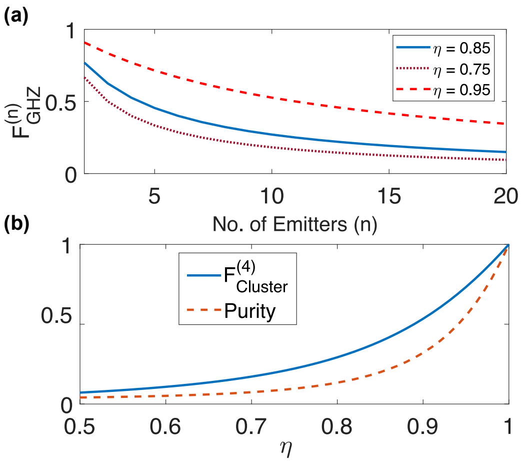


FIG. S4. (a) Fidelity of GHZ state generation for different number of spin emitters at three different efficiencies $\eta$. (b) Fidelity and purity of the heralded four-qubit cluster state as a function of $\eta$.

generate $N$-photon GHZ or cluster states [4]. While proposals for multi-photon entanglement using SiC defects have been put forward using photonic polarization states of the emitted photon [5], we focus here on the generation of another class of entangled states, the photon-number entangled states (PNES) [6].

For this let us consider a defect pair, whose spin-dependent transitions $A_1$ and $A_2$, similar to the experimentally observed defect pair shown in FIG. 3(a) in the main text. Initializing the two defects in their respective spin ground states $|\uparrow\uparrow\rangle$, followed by a MW $\pi/2$-pulse, allows the creation of an equal superposition state and upon excitation with a short laser pulse resonant with the central transition and restricting the photon detection basis to 0 and 1, we have a spin-photon entangled state:

$$|\psi_{12}\rangle = \frac{1}{2}\Big(\frac{1}{\sqrt{2}}[|\uparrow_1\uparrow_2\rangle + |\downarrow_1\downarrow_2\rangle]|1\rangle + |\downarrow_1\uparrow_2\rangle|0\rangle + |\uparrow_1\downarrow_2\rangle|2\rangle\Big) \tag{S3}$$

By repeating the excitation process with a resonant laser pulse at the same energy, we add photons onto the respective spin states from these different excitation pulses (delayed in time)

$$|\psi_{12}\rangle = \frac{1}{2}(\frac{1}{\sqrt{2}}[|\uparrow_1\uparrow_2\rangle + |\downarrow_1\downarrow_2\rangle]|1\rangle_E|1\rangle_L + |\downarrow_1\uparrow_2\rangle|0\rangle_E|0\rangle_L + |\uparrow_1\downarrow_2\rangle|2\rangle_E|2\rangle_L), \tag{S4}$$

where in the above $E$, $L$ represent the early and late photon emission events. By performing a MW $\pi/2$-pulse and projecting them onto their initial state, we obtain the the resulting state of the photons, given by

$$|n\rangle_1 = C_0|0\rangle_E|0\rangle_L + C_1|1\rangle_E|1\rangle_L + C_2|2\rangle_E|2\rangle_L \tag{S5}$$

We would like to note that the coefficients $C_k$ can be chosen with the choice of the initial and final MW pulses applied on the spin states of both the defects. For example a choice of $C_0 \approx 0.765$, $C_1 \approx 0.535, C_2 \approx 0.359$, is shown to lead to maximal Bell correlations and two-mode squeezing of $\sim 3\,\text{dB}$ [6].

* f.kaiser@pi3.uni-stuttgart.de

[1] R. Von Mises and G. Birkhoff, *Selected Papers of Richard von Mises*. No. Bd. 1 in Selected Papers, American Mathematical Society, 1963.
[2] R. Nagy, M. Niethammer, M. Widmann, Y.-C. Chen, P. Udvarhelyi, C. Bonato, J. U. Hassan, R. Karhu, I. G. Ivanov, N. T. Son, J. R. Maze, T. Ohshima, Ö. O. Soykal, Á. Gali, S.-Y. Lee, F. Kaiser, and J. Wrachtrup, "High-fidelity spin and optical control of single silicon-vacancy centres in silicon carbide," *Nature Communications*, vol. 10, no. 1, p. 1954, 2019.
[3] K. Chen, C.-M. Li, Q. Zhang, Y.-A. Chen, A. Goebel, S. Chen, A. Mair, and J.-W. Pan, "Experimental realization of one-way quantum computing with two-photon four-qubit cluster states," *Physical Review Letters*, vol. 99, p. 120503, Sep 2007.
[4] D. D. B. Rao, S. Yang, and J. Wrachtrup, "Generation of entangled photon strings using nv centers in diamond," *Physical Review B*, vol. 92, p. 081301, Aug 2015.
[5] S. E. Economou, N. Lindner, and T. Rudolph, "Optically generated 2-dimensional photonic cluster state from coupled quantum dots," *Physical Review Letters*, vol. 105, no. 9, p. 093601, 2010.
[6] S.-Y. Lee, J. Park, H.-W. Lee, and H. Nha, "Generating arbitrary photon-number entangled states for continuous-variable quantum informatics," *Optics Express*, vol. 20, pp. 14221–14233, Jun 2012.
